# Supplementary material for: AdvFusion: Adapter-based Knowledge Transfer for Code Summarization on Code Language Models
Source: arXiv:2307.07854 source file (2024-12-21)
Supplement: Supplementary file 1 [file appendix.tex]

\section{Appendix}
\subsection{AdvFusion contribution on other languages}

\begin{figure}
\includegraphics[width=\columnwidth]{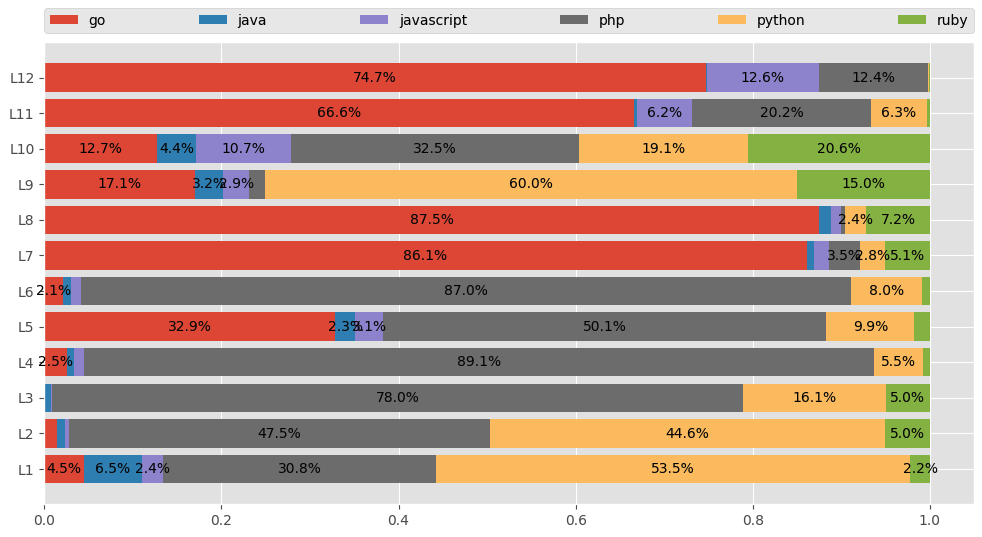}
\centering
\caption{The attention contribution from each programming language at each layer when we feed the Go test dataset to the fine-tuned AdapterFusion model.}
\label{fig:fusion-go}
\end{figure}

\begin{figure}
\includegraphics[width=\columnwidth]{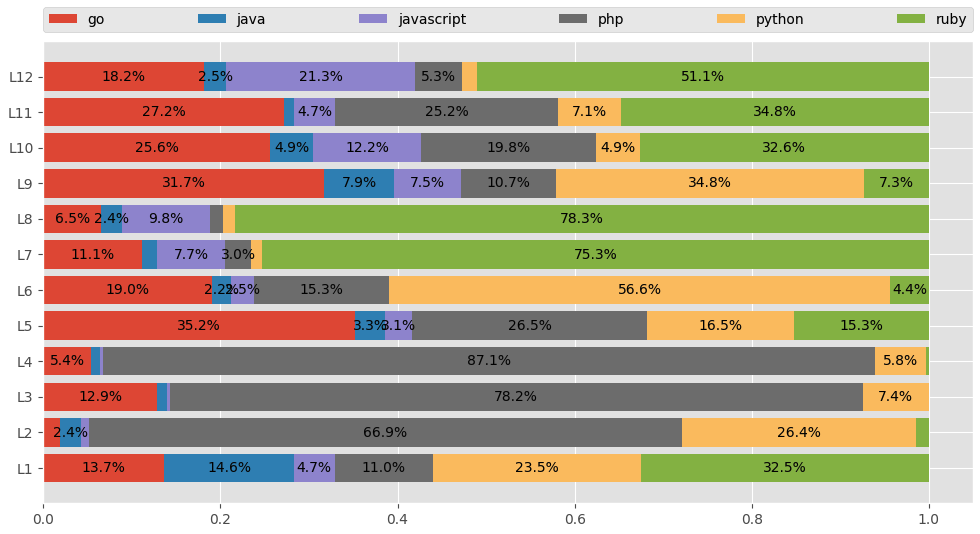}
\centering
\caption{The attention contribution from each programming language at each layer when we feed the Go test dataset to the fine-tuned AdvFusion model.}
\label{fig:adv-fusion-go}
\end{figure}

\begin{figure}
\includegraphics[width=\columnwidth]{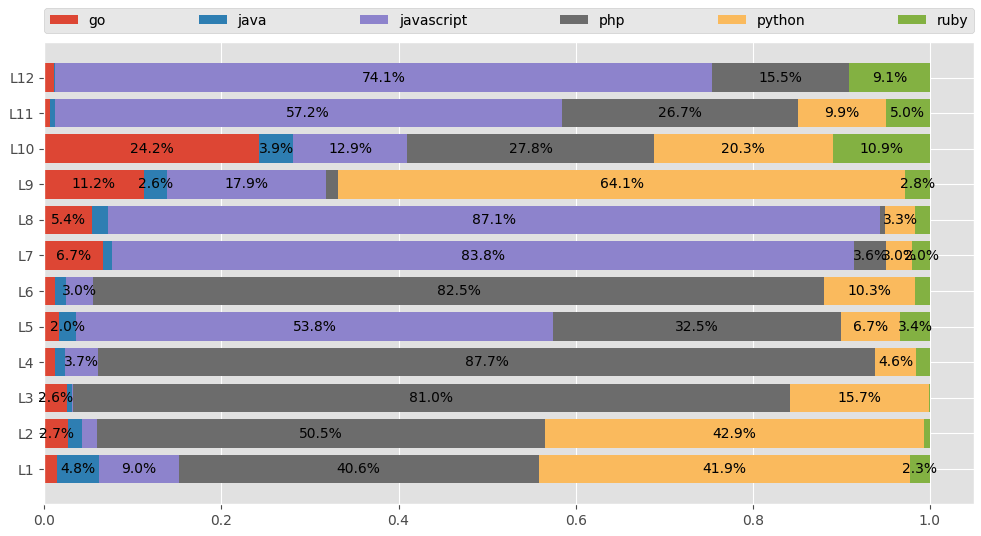}
\centering
\caption{The attention contribution from each programming language at each layer when we feed the JavaScript test dataset to the fine-tuned AdapterFusion model.}
\label{fig:fusion-go}
\end{figure}

\begin{figure}
\includegraphics[width=\columnwidth]{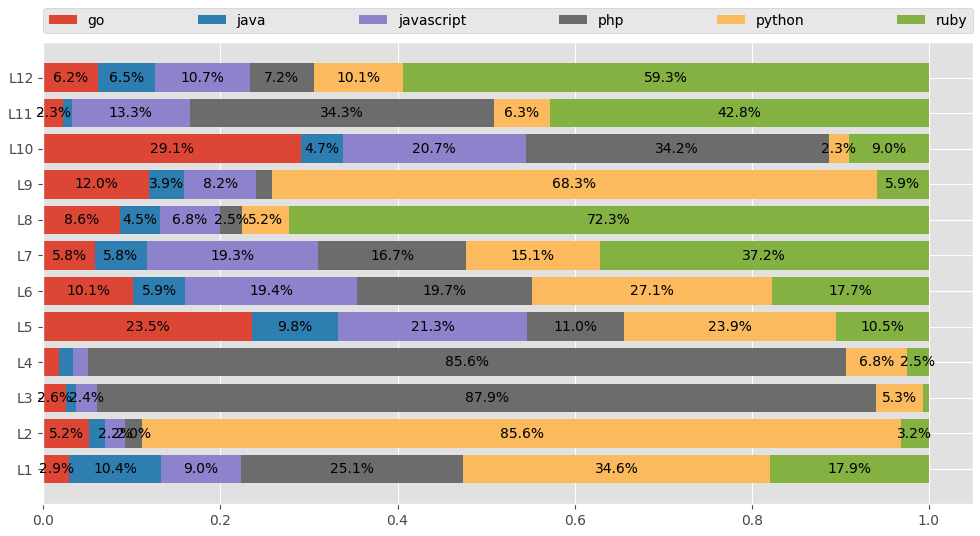}
\centering
\caption{The attention contribution from each programming language at each layer when we feed the JavaScript test dataset to the fine-tuned AdvFusion model.}
\label{fig:adv-fusion-go}
\end{figure}

\begin{figure}
\includegraphics[width=\columnwidth]{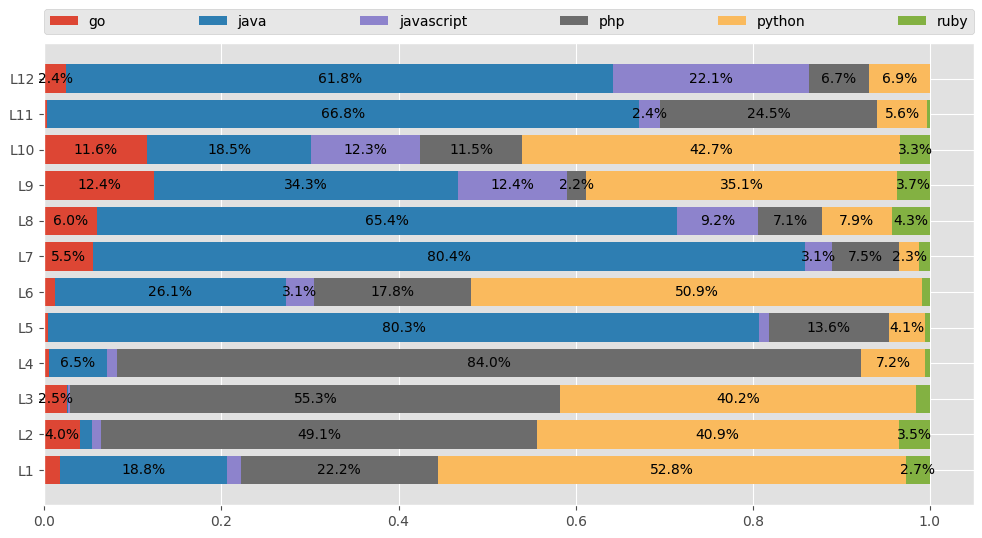}
\centering
\caption{The attention contribution from each programming language at each layer when we feed the Java test dataset to the fine-tuned AdapterFusion model.}
\label{fig:fusion-go}
\end{figure}

\begin{figure}
\includegraphics[width=\columnwidth]{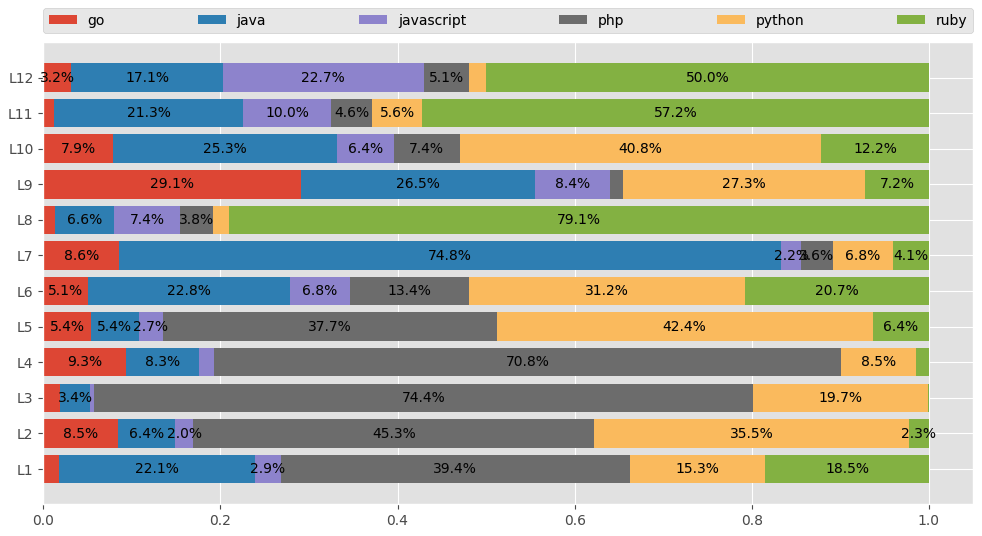}
\centering
\caption{The attention contribution from each programming language at each layer when we feed the Java test dataset to the fine-tuned AdvFusion model.}
\label{fig:adv-fusion-go}
\end{figure}
